# Supplementary material for: Efficient Reactive Synthesis Using Mode Decomposition
Source: arXiv:2312.08717 source file (2023-12-14)
Supplement: Supplementary file 1 [file appendix.tex]

\section{Appendix}
\label{appendix}
This section contains the proofs of the results stated in this paper.
\subsection{Proof Lemma~\ref{}}
Given a set of projections $P =\{p_1,\ldots,p_k\}$, 
% a set of modes $M = \{m_1,\ldots,m_k\}$, and a set of jumping conditions $J = \{j_1,\ldots,j_k\}$, 
if each projection $p_i \in P$ is realizable, then the original specification $\varphi$ if realizable.
\begin{proof}[Lemma~\ref{}]
    Suppose by
\end{proof}
